# Supplementary material for: From the betweenness centrality in street networks to structural invariants in random planar graphs
Source: arXiv:1709.05718 ancillary file (2018-07-02)
Supplement: Supplementary file 1 [file SI_v3.pdf]

# Supporting Information

**From the betweenness centrality in street networks to structural invariants in random planar graphs**

Alec Kirkley, Hugo Barbosa, Marc Barthelemy, Gourab Ghoshal

## S1 Data

Raw shapefile data for the street geometries and locations was collected from the OpenStreetMaps (OSM) database [1]. For each city we extracted the geospatial vector data of the roads within a bounding box circumscribing an area of 30 km radius from the city centers. The 30km radius was chosen to encapsulate both high density urban regions and more suburban regions with fewer, longer streets. After aggregating all the raw shapefile data, we populated the Rtree data structure with the linestring (a collection of latitude/longitude coordinates approximating the contour of the street) geometry of each street.

Then, for each street, we found the other streets intersecting it using the Rtree indexing, and cut the street into separate segments at each intersection point, adding a node at each of these points. Latitude and longitude coordinates of all nodes were projected onto global distances using the Mercator projection, and then an edge was added between nodes adjacent along a given street, with a weight equal to the Euclidean distance between the nodes. After searching through all streets, and checking for connectivity, the street networks were complete. The type of each street, classified into various categories by OSM ('Motorway', 'Primary', 'Service', etc.), was then added as an attribute to each edge, and two versions of the street network were created for each city. For each city, the entire street network was created, and in addition, a "refined" street network was created to approximate the network of high congestion streets, where only edges classified as primary, secondary, tertiary, highways, or service roads were kept, and all others were pruned, then the giant component of the resulting network was kept. All analyses were performed on the entire street network, except for the randomized cities analyses (i.e. randomizing the weights, rewiring the edges, etc), which were done on the filtered street networks for computational tractability. Descriptive statistics for the entire street networks of individual cities are shown in Table S1.

It is noteworthy that in our data, individual roads are represented as single edges, regardless of the number of traffic lanes. Roads with two or more roadways with a physical barrier separating the traffic directions (e.g., divided highways and expressways) will have one edge for each physical roadway.

Table S1: Statistics of the street networks sorted by number of nodes $N$ (i.e., intersection). The total length $\ell$ corresponds to the sum of the lengths of all streets within a convex hull of area $A$.

| City | Nodes $N$ | Edges $e$ | Length $\ell$ (km) | Area $A$ (km$^2$) | Density $\rho$ |
|---|---|---|---|---|---|
| Tokyo | 612418 | 976040 | 82586.30 | 6552.04 | 93.47 |
| Moscow | 307472 | 482217 | 61391.85 | 11562.73 | 26.59 |
| Nagoya | 300588 | 496495 | 57990.36 | 5891.78 | 51.02 |
| Osaka | 292855 | 469333 | 47827.03 | 5968.06 | 49.07 |
| Paris | 279072 | 425108 | 57285.37 | 8911.36 | 31.32 |
| Milan | 201029 | 299564 | 38929.31 | 8412.68 | 23.90 |
| Berlin | 198498 | 306742 | 49006.85 | 10027.52 | 19.80 |
| Washington DC | 183687 | 276391 | 35296.45 | 6464.47 | 28.41 |
| São Paulo | 180843 | 283349 | 32579.38 | 5619.28 | 32.18 |
| New York City | 178120 | 288278 | 43137.88 | 6729.33 | 26.47 |
| Madrid | 177403 | 273342 | 33647.67 | 6119.91 | 28.99 |
| Houston | 175524 | 270779 | 34352.18 | 5278.51 | 33.25 |
| Delhi | 174732 | 267204 | 30124.32 | 6127.09 | 28.52 |
| Los Angeles | 166993 | 268304 | 38984.48 | 4866.74 | 34.31 |
| Alexandria | 162753 | 244978 | 31964.20 | 6371.30 | 25.54 |
| Mexico City | 158528 | 254762 | 27406.55 | 4436.46 | 35.73 |
| Chicago | 157740 | 258044 | 34761.24 | 3992.69 | 39.51 |
| Toronto | 156919 | 248099 | 27457.24 | 4307.80 | 36.43 |
| Phoenix | 153846 | 235348 | 32294.83 | 6097.68 | 25.23 |
| Hyderabad | 151131 | 231787 | 19793.77 | 4471.25 | 33.80 |
| Istanbul | 149511 | 235069 | 24757.37 | 4127.72 | 36.22 |
| Buenos Aires | 138245 | 241717 | 29794.35 | 3063.27 | 45.13 |
| Philadelphia | 122916 | 192174 | 31816.90 | 6252.88 | 19.66 |
| Khartoum | 122634 | 200241 | 16405.95 | 2972.44 | 41.26 |
| Manila | 118712 | 178773 | 16436.52 | 3031.90 | 39.15 |
| Boston | 118573 | 177186 | 28054.72 | 6991.56 | 16.96 |
| Barcelona | 110982 | 172526 | 23751.22 | 4073.86 | 27.24 |
| London | 105198 | 139541 | 25931.41 | 9401.36 | 11.19 |
| Lima | 99750 | 160214 | 13356.04 | 1841.42 | 54.17 |
| Riyadh | 98569 | 151902 | 20417.77 | 3800.11 | 25.94 |
| Atlanta | 92148 | 131969 | 23421.24 | 5949.59 | 15.49 |

Continued on next page

| City | Nodes $N$ | Edges $e$ | Length $\ell$ (km) | Area $A$ (km$^2$) | Density $\rho$ |
|---|---|---|---|---|---|
| Kuala Lumpur | 89879 | 133348 | 16412.21 | 3777.69 | 23.79 |
| Rome | 86374 | 129451 | 19242.76 | 6093.85 | 14.17 |
| San Francisco | 85635 | 135493 | 18801.50 | 4855.68 | 17.64 |
| Sydney | 82870 | 123436 | 17758.48 | 3273.63 | 25.31 |
| Rio De Janeiro | 82808 | 129256 | 15711.31 | 2956.19 | 28.01 |
| Johannesburg | 78377 | 121053 | 21198.68 | 5231.78 | 14.98 |
| Jakarta | 74128 | 112467 | 12520.81 | 2484.23 | 29.84 |
| Taipei | 74105 | 118000 | 15001.50 | 3834.81 | 19.32 |
| Monterrey | 73981 | 117784 | 12812.46 | 3724.65 | 19.86 |
| Bangalore | 73759 | 112712 | 13753.09 | 3966.04 | 18.60 |
| Bogota | 73648 | 117684 | 11133.31 | 3927.02 | 18.75 |
| Miami | 72411 | 115085 | 15548.93 | 2186.57 | 33.12 |
| Bangkok | 71582 | 102908 | 16316.54 | 4170.52 | 17.16 |
| Cairo | 70777 | 109185 | 16406.14 | 5653.43 | 12.52 |
| Guadalajara | 70145 | 113418 | 12226.81 | 5873.67 | 11.94 |
| Shenzhen | 65286 | 101370 | 14927.35 | 3810.12 | 17.13 |
| Dubai | 62559 | 91822 | 12126.64 | 2478.23 | 25.24 |
| Hong Kong | 62451 | 96059 | 11831.31 | 2716.85 | 22.99 |
| Ankara | 61133 | 95797 | 13571.78 | 5673.95 | 10.77 |
| Tehran | 57177 | 88127 | 12898.16 | 4411.81 | 12.96 |
| Cape Town | 52096 | 78827 | 10794.67 | 2460.27 | 21.17 |
| Shanghai | 50049 | 82637 | 19566.98 | 5539.79 | 9.03 |
| Chennai | 49278 | 74444 | 8786.05 | 2181.86 | 22.59 |
| Baghdad | 48271 | 75255 | 10837.62 | 4839.89 | 9.97 |
| Santiago | 43001 | 64873 | 18578.85 | 6824.06 | 6.30 |
| Yangon | 40840 | 64890 | 7689.51 | 3418.27 | 11.95 |
| Kolkata | 38924 | 57162 | 7258.99 | 3663.49 | 10.62 |
| Ho Chi Minh City | 38311 | 58902 | 9277.30 | 3679.66 | 10.41 |
| Guangzhou | 35921 | 57460 | 14606.66 | 5447.64 | 6.59 |
| Luanda | 35468 | 57329 | 7934.13 | 2101.68 | 16.88 |
| Mumbain | 32720 | 49535 | 7182.38 | 2772.80 | 11.80 |
| Singapore | 29756 | 44640 | 5317.58 | 777.07 | 38.29 |
| Lahore | 28008 | 43723 | 7509.84 | 4821.33 | 5.81 |
| Surabaya | 26420 | 39506 | 5467.28 | 2964.76 | 8.91 |
| Abidjan | 24499 | 37922 | 4564.90 | 2713.18 | 9.03 |
| Melbourne | 22287 | 33817 | 5789.36 | 3330.35 | 6.69 |
| Kinshasa | 21711 | 35563 | 4108.92 | 1624.39 | 13.37 |
| Accra | 21333 | 32060 | 5346.94 | 2062.73 | 10.34 |
| Dar es Salaam | 20754 | 31061 | 3564.65 | 2073.43 | 10.01 |
| Dongguan | 19294 | 31452 | 10738.15 | 5769.56 | 3.34 |
| Lagos | 18936 | 28066 | 5084.47 | 2406.29 | 7.87 |
| Xian | 18925 | 30592 | 12378.79 | 7923.66 | 2.39 |
| Nanjing | 17500 | 28518 | 9911.60 | 6192.78 | 2.83 |

Continued on next page

| City | Nodes $N$ | Edges $e$ | Length $\ell$ (km) | Area $A$ (km$^2$) | Density $\rho$ |
|---|---|---|---|---|---|
| Nairobi | 17040 | 24463 | 5529.59 | 3184.32 | 5.35 |
| Bandung | 16755 | 24529 | 3715.87 | 3939.03 | 4.25 |
| Wuhan | 16568 | 26508 | 8629.57 | 6446.66 | 2.57 |
| Pune | 16173 | 23905 | 4800.26 | 3905.53 | 4.14 |
| Tianjin | 15461 | 25641 | 10362.45 | 7058.71 | 2.19 |
| Hanoi | 14864 | 22934 | 5505.63 | 4592.05 | 3.24 |
| Hangzhou | 14829 | 24512 | 8933.17 | 5644.03 | 2.63 |
| Kabul | 14137 | 21517 | 3931.07 | 2919.67 | 4.84 |
| Ahmadabad | 13615 | 21046 | 4465.10 | 3988.31 | 3.41 |
| Chengdu | 12521 | 20724 | 7967.42 | 5327.72 | 2.35 |
| Suzhou | 12501 | 21104 | 9317.10 | 4952.66 | 2.52 |
| Dhaka | 12209 | 18423 | 3427.93 | 4836.00 | 2.52 |
| Medan | 10424 | 15660 | 2964.14 | 1749.25 | 5.96 |
| Xiamen | 9679 | 15652 | 4598.72 | 3758.04 | 2.58 |
| Shenyang | 9624 | 15853 | 7538.69 | 6475.61 | 1.49 |
| Chongqing | 8275 | 13232 | 5133.81 | 4740.14 | 1.75 |
| Qingdao | 7095 | 11911 | 4470.93 | 3476.07 | 2.04 |
| Fuzhou | 6310 | 9945 | 4519.80 | 4750.16 | 1.33 |
| Harbin | 6074 | 9990 | 4346.88 | 5059.06 | 1.20 |
| Dalian | 5654 | 9122 | 2989.32 | 2521.05 | 2.24 |
| Kuwait | 4593 | 6501 | 1826.65 | 4595.19 | 1.00 |
| Quangzhou | 3774 | 6189 | 3559.67 | 3248.89 | 1.16 |
| Surat | 3349 | 5020 | 1793.45 | 2635.62 | 1.27 |

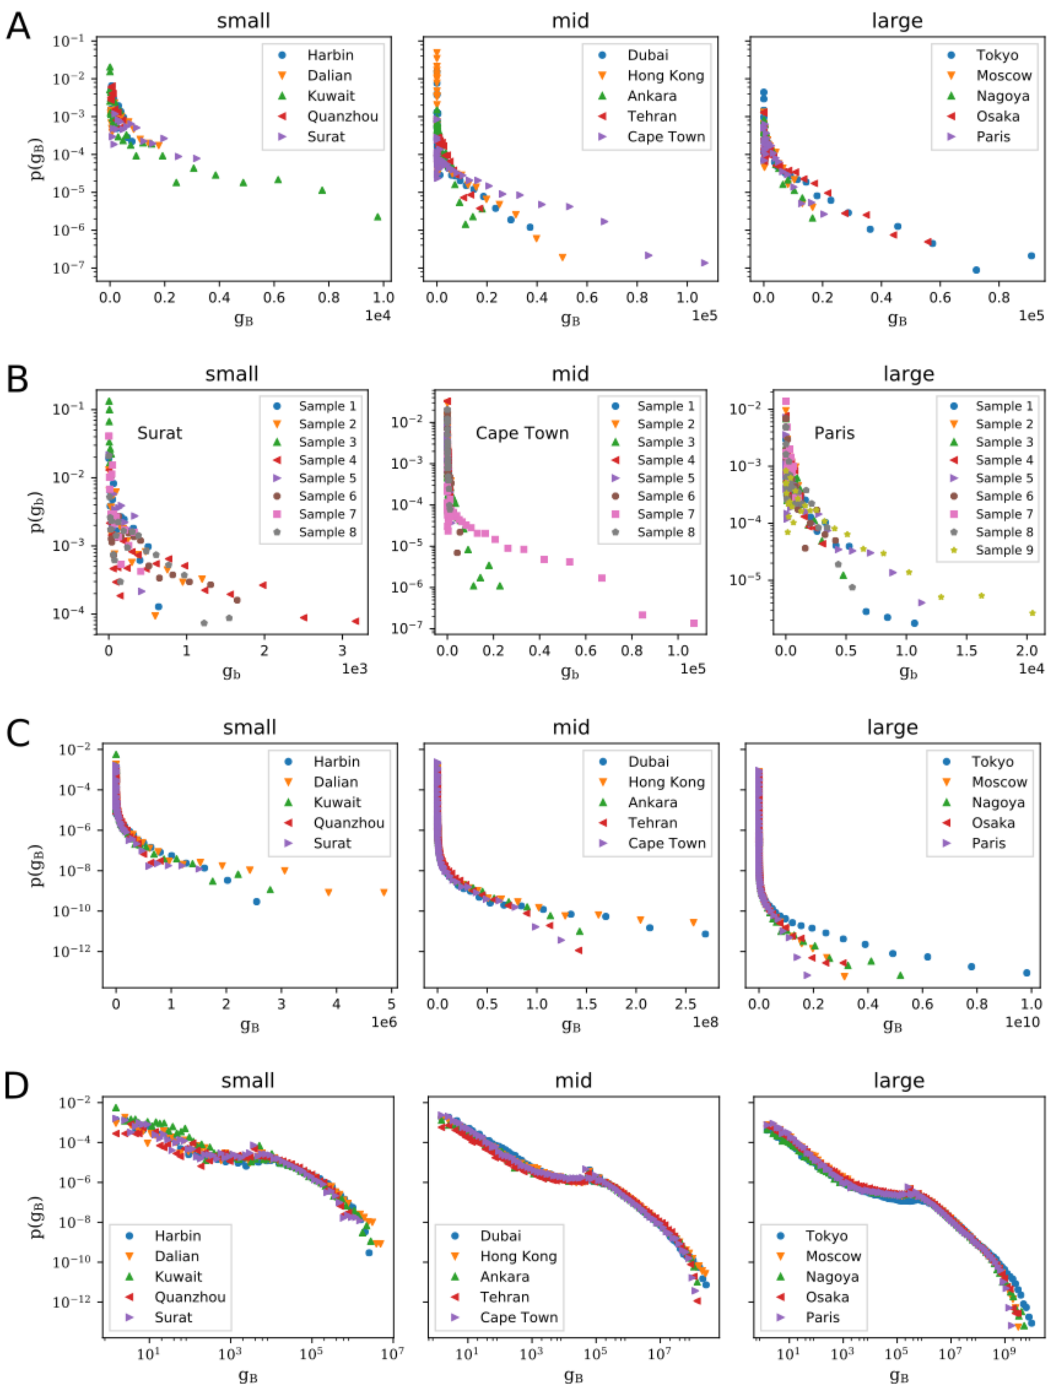


Figure S1: Betweenness pdf's at multiple scales (A) selected one-square-mile samples from each category (log-linear). (B) Multiple one-square-mile samples within a single city picked from each category (log-linear). (C) BC of streets at full resolution $\sim$ 1000 square-miles (log-linear) and finally (D) the same in log-log scale revealing a bimodal distribution.

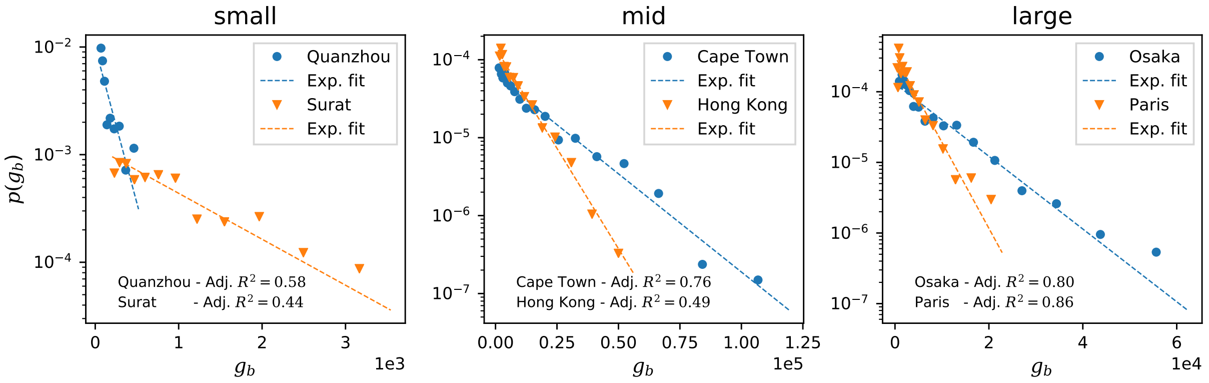


Figure S2: Distribution of $g_B$ for 1sq mile samples for cities of different network sizes and their corresponding exponential fits.

## S2 Curve fitting and verification

Curve fits were performed using the maximum likelihood procedures outlined in [2]. As we show in the main document, the tails of the BC distributions are well approximated by a truncated power-law distribution

$$p(\tilde{g}_B) \sim \tilde{g}_B^{-\alpha} e^{-\tilde{g}_B/\beta}.$$

Figure S3 shows the tail of the BC distributions with their corresponding fit lines whereas Table S2 shows the results of the curve fits for each individual city. Additionally, we fit the tails to stretched exponentials of the form

$$p(\tilde{g}_B) \sim \tilde{g}_B^{\gamma-1} e^{-\lambda(\tilde{g}_B)^\gamma}.$$

Fits for $\gamma$ revealed a tightly peaked distribution near $\gamma \sim .3$ for all cities. This indicates that regardless of the exact functional form of the decay, the same power law scaling exponent of $\sim -1$ persists throughout all cities, with some variation that gets absorbed into the functional form of the tail decay, which is consistent with calculations for the Cayley Tree with fixed branching ratio. Therefore only the results for the truncated power law are reported in the manuscript as the exact functional form of the tails is not germane to the main discussion.

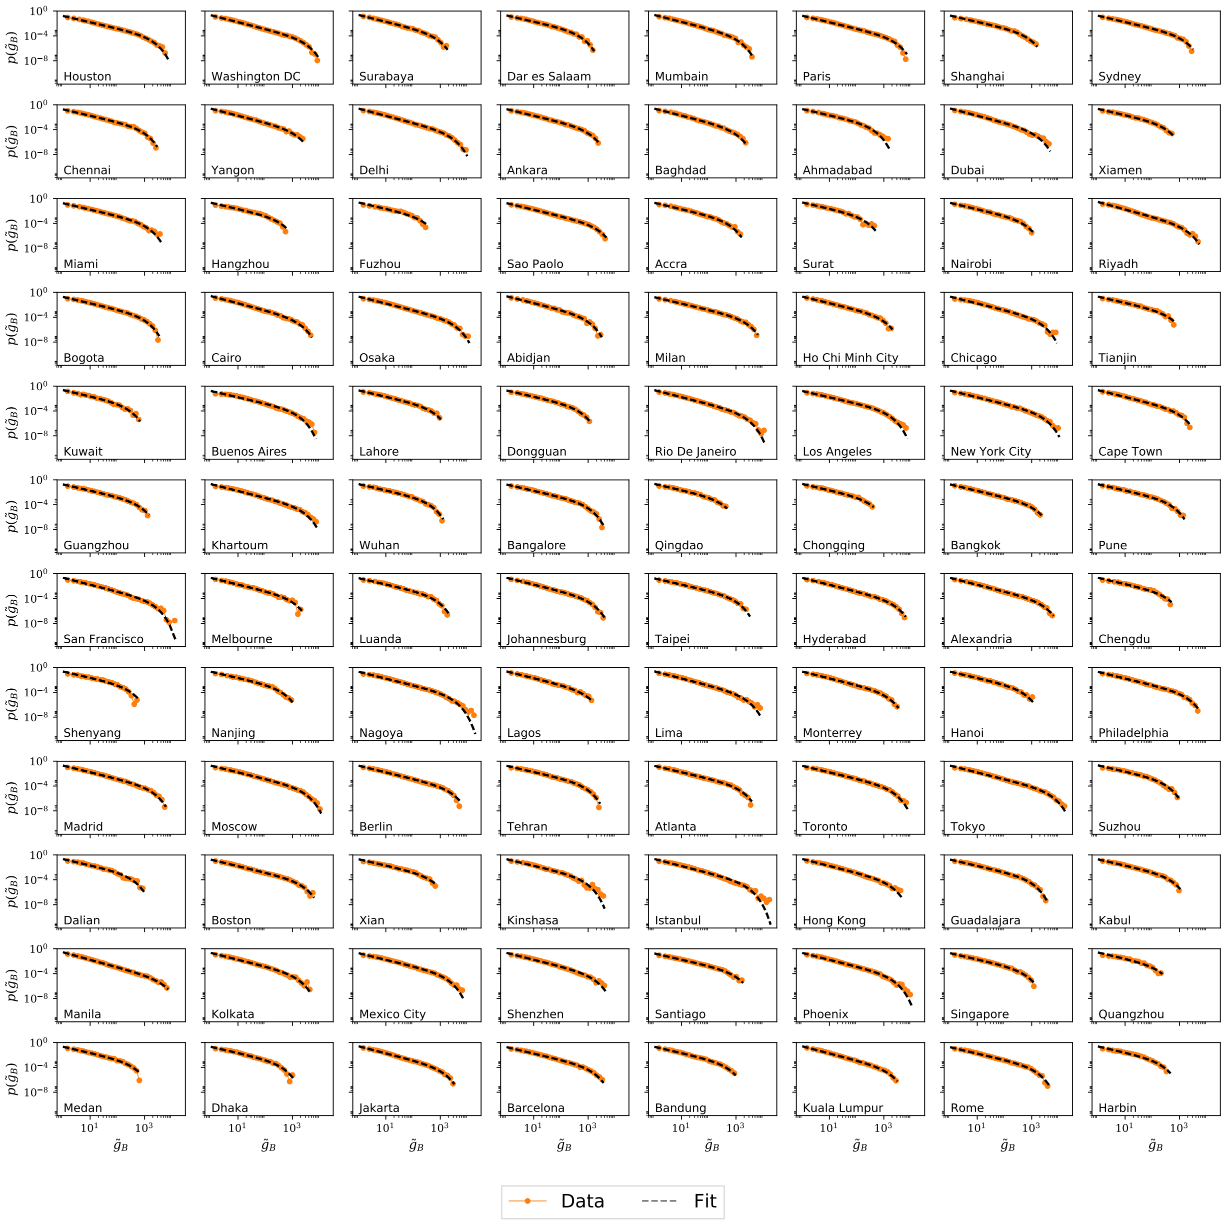


Figure S3: Tails of the BC distributions with their corresponding truncated-power-law fits for all cities, in no particular order.

Table S2: Parameter values for the truncated power law distributions fitted to the data.

| City | $\alpha$ | $\beta$ |
|---|---|---|
| Los Angeles | $1.000 \pm 0.002$ | 833.56 |
| Santiago | $1.000 \pm 0.003$ | 533.34 |
| Shanghai | $1.000 \pm 0.003$ | 386.91 |
| Tehran | $1.000 \pm 0.003$ | 451.24 |
| Taipei | $1.000 \pm 0.003$ | 544.44 |
| Guangzhou | $1.000 \pm 0.004$ | 349.23 |
| Luanda | $1.000 \pm 0.004$ | 372.26 |
| Singapore | $1.000 \pm 0.005$ | 311.91 |
| Xian | $1.000 \pm 0.005$ | 246.95 |
| Pune | $1.000 \pm 0.006$ | 267.52 |
| Wuhan | $1.000 \pm 0.006$ | 222.75 |
| Hangzhou | $1.000 \pm 0.006$ | 199.18 |
| Dongguan | $1.000 \pm 0.006$ | 259.99 |
| Tianjin | $1.000 \pm 0.006$ | 228.69 |
| Nanjing | $1.000 \pm 0.006$ | 230.24 |
| Dar es Salaam | $1.000 \pm 0.006$ | 285.57 |
| Chengdu | $1.000 \pm 0.007$ | 183.08 |
| Suzhou | $1.000 \pm 0.007$ | 175.23 |
| Kabul | $1.000 \pm 0.007$ | 261.67 |
| Dhaka | $1.000 \pm 0.007$ | 228.10 |
| Ahmadabad | $1.000 \pm 0.007$ | 214.40 |
| Medan | $1.000 \pm 0.008$ | 206.62 |
| Shenyang | $1.000 \pm 0.008$ | 156.62 |

Continued on next page

| City | $\alpha$ | $\beta$ |
|---|---|---|
| Xiamen | $1.000 \pm 0.009$ | 166.57 |
| Chongqing | $1.000 \pm 0.009$ | 168.52 |
| Fuzhou | $1.000 \pm 0.010$ | 133.97 |
| Qingdao | $1.000 \pm 0.010$ | 159.30 |
| Harbin | $1.000 \pm 0.011$ | 121.43 |
| Dalian | $1.000 \pm 0.012$ | 181.44 |
| Quangzhou | $1.000 \pm 0.014$ | 93.07 |
| Kuwait | $1.000 \pm 0.015$ | 134.41 |
| Surat | $1.000 \pm 0.016$ | 116.08 |
| Buenos Aires | $1.001 \pm 0.002$ | 816.10 |
| Houston | $1.008 \pm 0.002$ | 1044.60 |
| Guadalajara | $1.009 \pm 0.003$ | 516.32 |
| Bangalore | $1.012 \pm 0.003$ | 534.41 |
| Bandung | $1.013 \pm 0.007$ | 268.97 |
| Nairobi | $1.015 \pm 0.007$ | 301.92 |
| Hanoi | $1.015 \pm 0.007$ | 267.13 |
| Chennai | $1.018 \pm 0.003$ | 501.82 |
| Bogota | $1.018 \pm 0.003$ | 556.28 |
| Lahore | $1.020 \pm 0.005$ | 286.75 |
| Sydney | $1.021 \pm 0.003$ | 736.42 |
| Accra | $1.023 \pm 0.006$ | 305.32 |
| Rome | $1.024 \pm 0.002$ | 782.85 |
| Miami | $1.025 \pm 0.003$ | 679.11 |
| Milan | $1.027 \pm 0.001$ | 1289.63 |
| Atlanta | $1.029 \pm 0.002$ | 808.04 |
| Barcelona | $1.031 \pm 0.002$ | 762.74 |

Continued on next page

| City | $\alpha$ | $\beta$ |
|---|---|---|
| Bangkok | $1.037 \pm 0.003$ | 677.47 |
| Kinshasa | $1.044 \pm 0.005$ | 417.81 |
| Paris | $1.047 \pm 0.001$ | 1418.81 |
| Toronto | $1.047 \pm 0.002$ | 1104.54 |
| Boston | $1.049 \pm 0.002$ | 1261.84 |
| Ankara | $1.051 \pm 0.003$ | 575.70 |
| Ho Chi Minh City | $1.052 \pm 0.004$ | 502.37 |
| Melbourne | $1.056 \pm 0.005$ | 558.14 |
| Mexico City | $1.057 \pm 0.002$ | 929.95 |
| Sao Paolo | $1.059 \pm 0.002$ | 1224.01 |
| Philadelphia | $1.061 \pm 0.002$ | 1036.82 |
| Berlin | $1.068 \pm 0.002$ | 1343.56 |
| New York City | $1.073 \pm 0.002$ | 1429.50 |
| Moscow | $1.077 \pm 0.001$ | 1480.18 |
| Madrid | $1.078 \pm 0.002$ | 1030.24 |
| Surabaya | $1.082 \pm 0.005$ | 391.68 |
| Chicago | $1.083 \pm 0.002$ | 1143.91 |
| Monterrey | $1.084 \pm 0.003$ | 735.52 |
| Nagoya | $1.087 \pm 0.001$ | 1560.92 |
| Johannesburg | $1.087 \pm 0.003$ | 698.69 |
| Lagos | $1.089 \pm 0.006$ | 456.59 |
| Kolkata | $1.092 \pm 0.004$ | 823.74 |
| Cape Town | $1.092 \pm 0.004$ | 565.36 |
| Shenzhen | $1.096 \pm 0.003$ | 868.03 |
| Osaka | $1.097 \pm 0.001$ | 1700.57 |
| Phoenix | $1.097 \pm 0.002$ | 1119.66 |

Continued on next page

| City | $\alpha$ | $\beta$ |
|---|---|---|
| Hyderabad | $1.097 \pm 0.002$ | 1323.22 |
| Khartoum | $1.100 \pm 0.002$ | 1262.22 |
| Tokyo | $1.101 \pm 0.001$ | 2698.20 |
| Abidjan | $1.101 \pm 0.005$ | 504.54 |
| Alexandria | $1.102 \pm 0.002$ | 1438.91 |
| San Francisco | $1.107 \pm 0.003$ | 1112.27 |
| Mumbain | $1.110 \pm 0.005$ | 662.04 |
| Hong Kong | $1.111 \pm 0.003$ | 921.48 |
| Baghdad | $1.113 \pm 0.004$ | 519.98 |
| Washington DC | $1.115 \pm 0.002$ | 1642.06 |
| Yangon | $1.117 \pm 0.004$ | 700.39 |
| Rio De Janeiro | $1.122 \pm 0.003$ | 1218.63 |
| Istanbul | $1.123 \pm 0.002$ | 1410.86 |
| Jakarta | $1.132 \pm 0.003$ | 672.21 |
| Lima | $1.139 \pm 0.002$ | 1236.50 |
| Kuala Lumpur | $1.140 \pm 0.003$ | 830.67 |
| Delhi | $1.150 \pm 0.002$ | 1393.89 |
| Cairo | $1.151 \pm 0.003$ | 957.97 |
| Dubai | $1.152 \pm 0.003$ | 783.79 |
| Riyadh | $1.205 \pm 0.003$ | 997.07 |
| Manila | $1.208 \pm 0.002$ | 2497.66 |

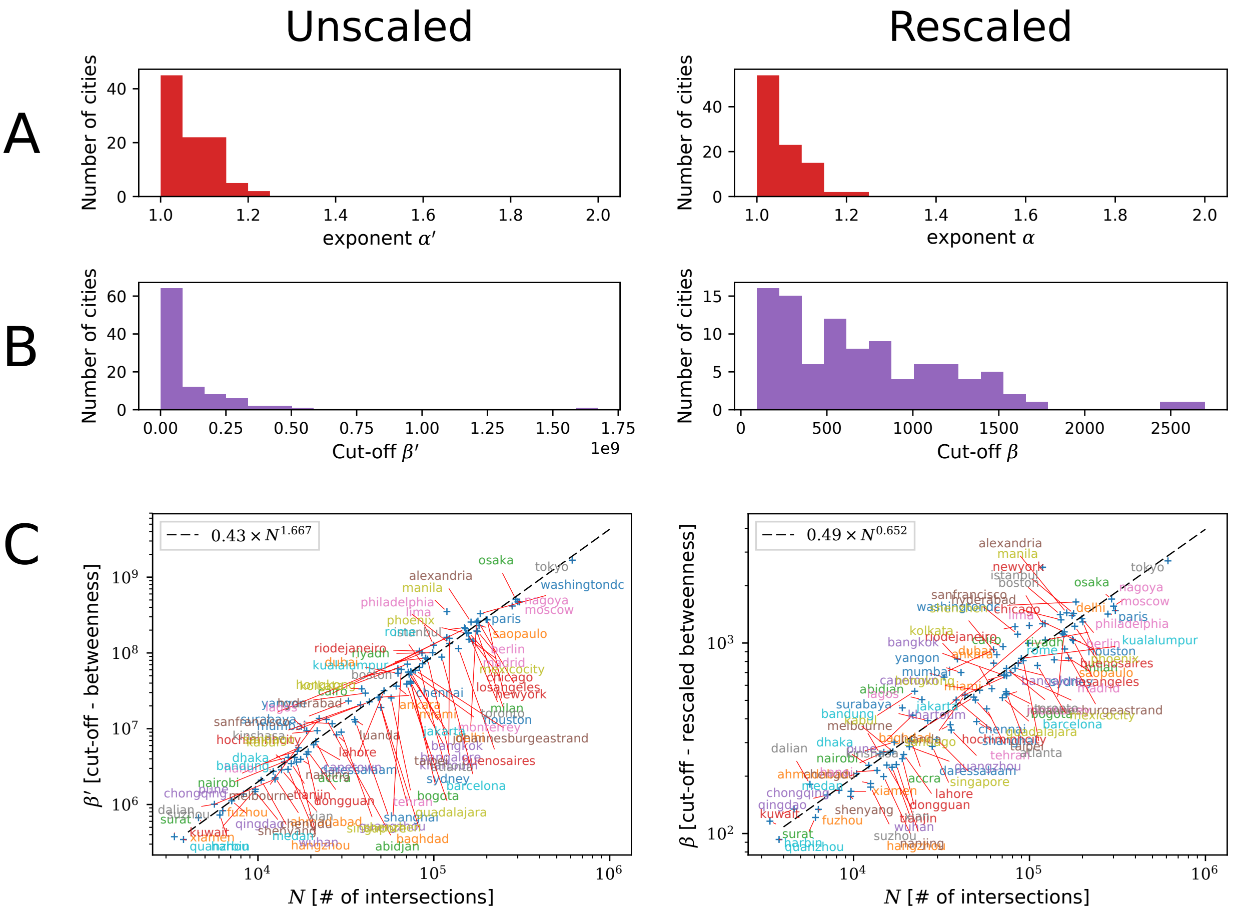


Figure S4: Distribution of the truncated-power-law parameters for both the unscaled (left panels) and rescaled BC (right panels). (A) The distribution of $\alpha$ is almost identical in both the rescaled and unscaled BC distributions. (B) The distribution of the exponential cut-off, $\beta$, changes dramatically from the unscaled to the rescaled versions of the BC. (C) These cut-offs also show a marked dependence on system size (number of nodes)

Figure S4 shows the distribution of power law exponents $\alpha, \alpha'$ and decay exponents $\beta, \beta'$ obtained for the tails of the betweenness distributions of all cities studied, both for the regular and rescaled betweenness. Also shown are the exponents $\beta, \beta'$ as a function of $N$.

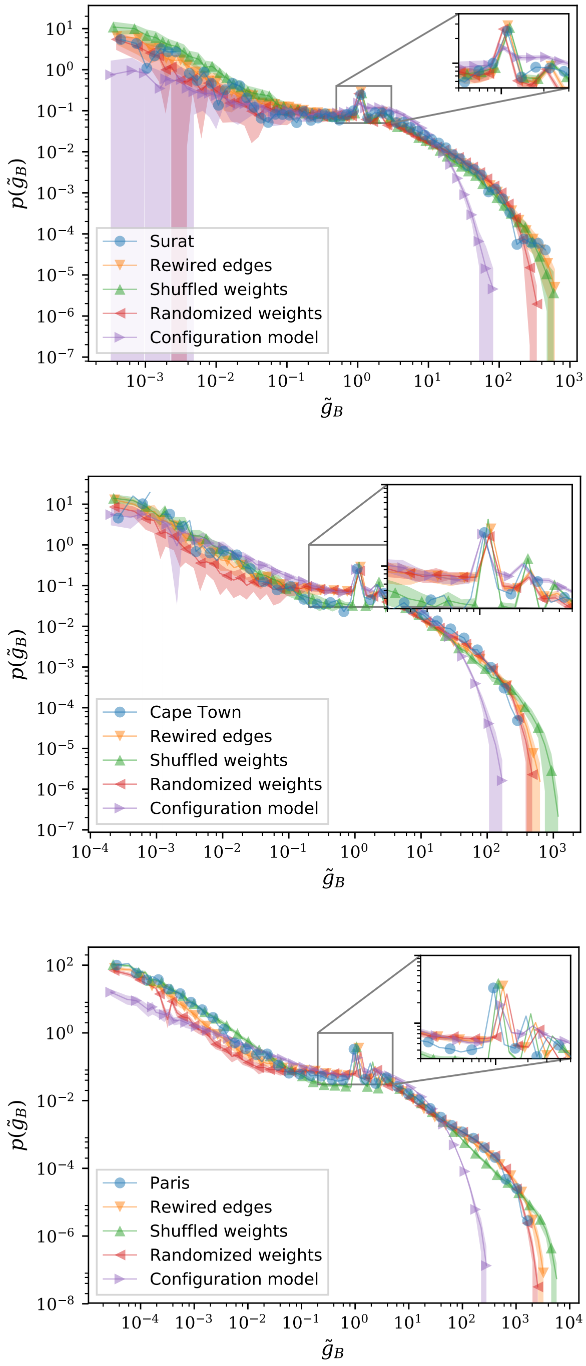


Figure S5: The BC distribution of various random graph models described in the main text compared to the baseline distribution of representative examples of cities of different sizes. Shaded area reflects fluctuations around the average over hundred realizations of each model.

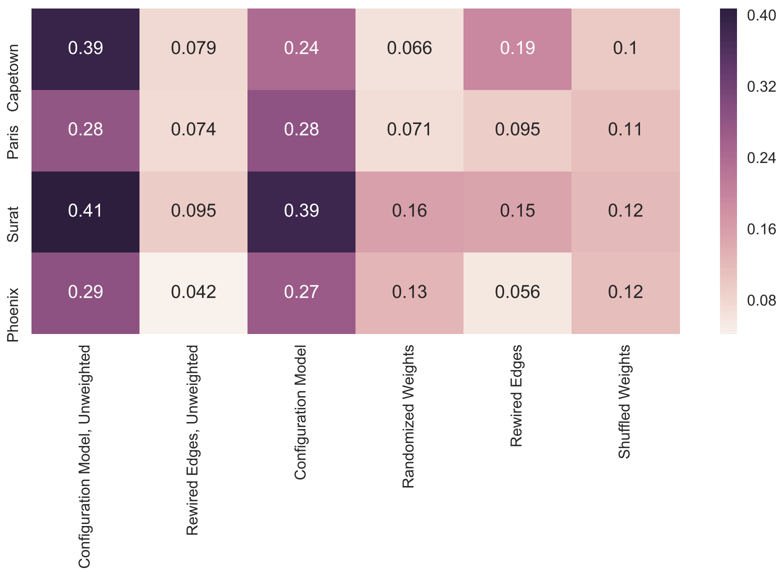


Figure S6: Average KS statistics over all 100 realizations of each random graph model when compared to the tail of the true betweenness distribution for cities at various size scales. In all cases, the non-planar configuration random graphs exhibit the most statistical dissimilarity from the original network in the tails of their betweenness distributions.

Figure S5 shows the betweenness distributions for the randomized versions of cities at various size scales in the same manner as what was done for Phoenix in Figure 2 in the main manuscript. The similarity in the distributions seen in that figure is replicated in these plots, and the corresponding 2-sample KS statistics for each random graph model (along with the unweighted versions of these simulations) are shown in S6 and S7. To obtain the reported values, the KS statistics were obtained for the comparison of the actual Phoenix street network tail (nodes with betweenness above $N$) and the tails of each of the 100 realizations of the given random graph model, which were then averaged to get a single value. Although the comparisons are not statistically significant for random graph models of large cities, we do see statistical significance in Surat, a much smaller city of 300 nodes, as well as for random samples from larger cities of sizes up to $\sim 500$ nodes. The KS statistic for the comparison of the street network with its non-planar configuration model counterpart is more than double that of the next highest KS value, indicating that the constraint of planarity has a much stronger effect on the betweenness distribution than other structural perturbations.

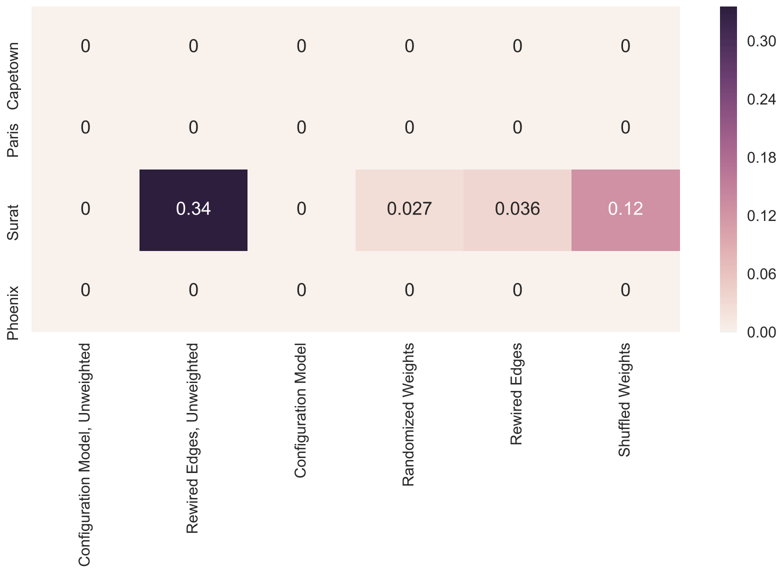


Figure S7: Average 2-sample KS p-values over all 100 realizations of each random graph model when compared to the tail of the true betweenness distribution for cities at various size scales.

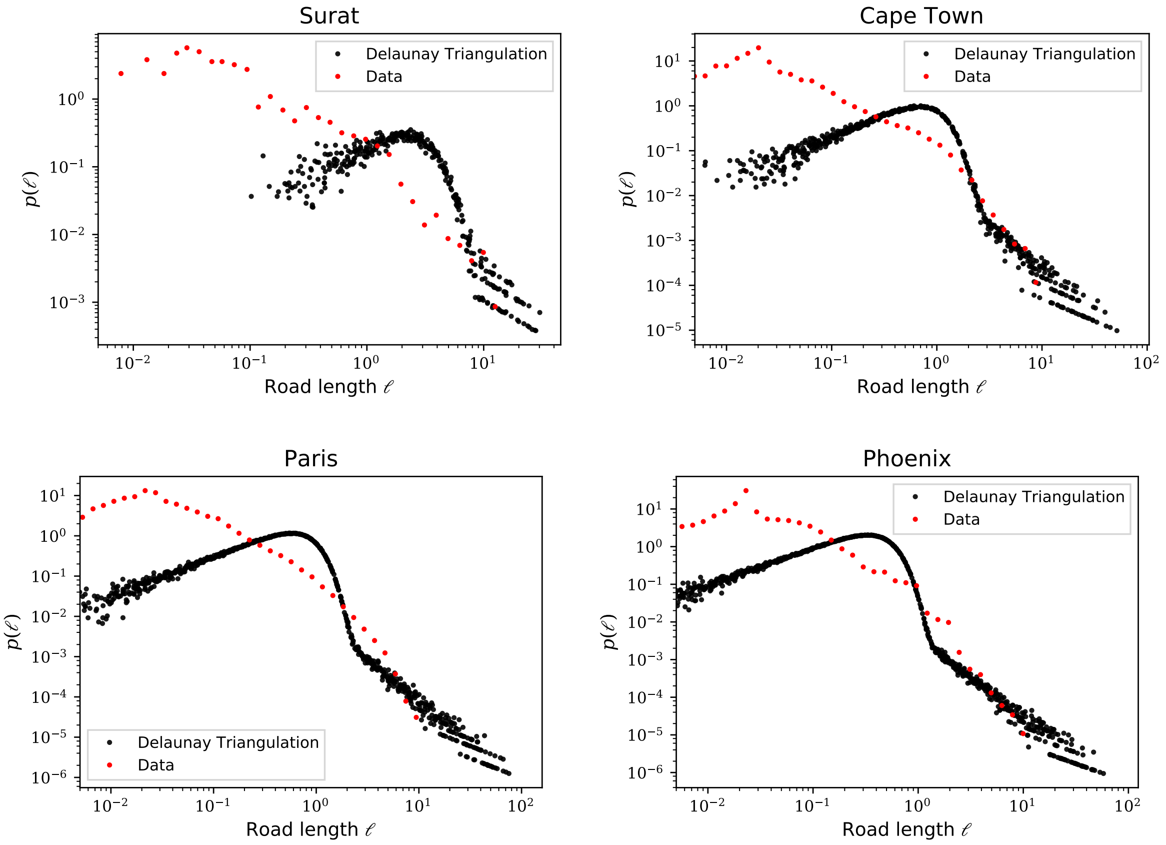


ca

Figure S8: Distribution of road segment lengths (in km) for three selected cities of different sizes along with the length distribution of their corresponding Delaunay Triangulations.

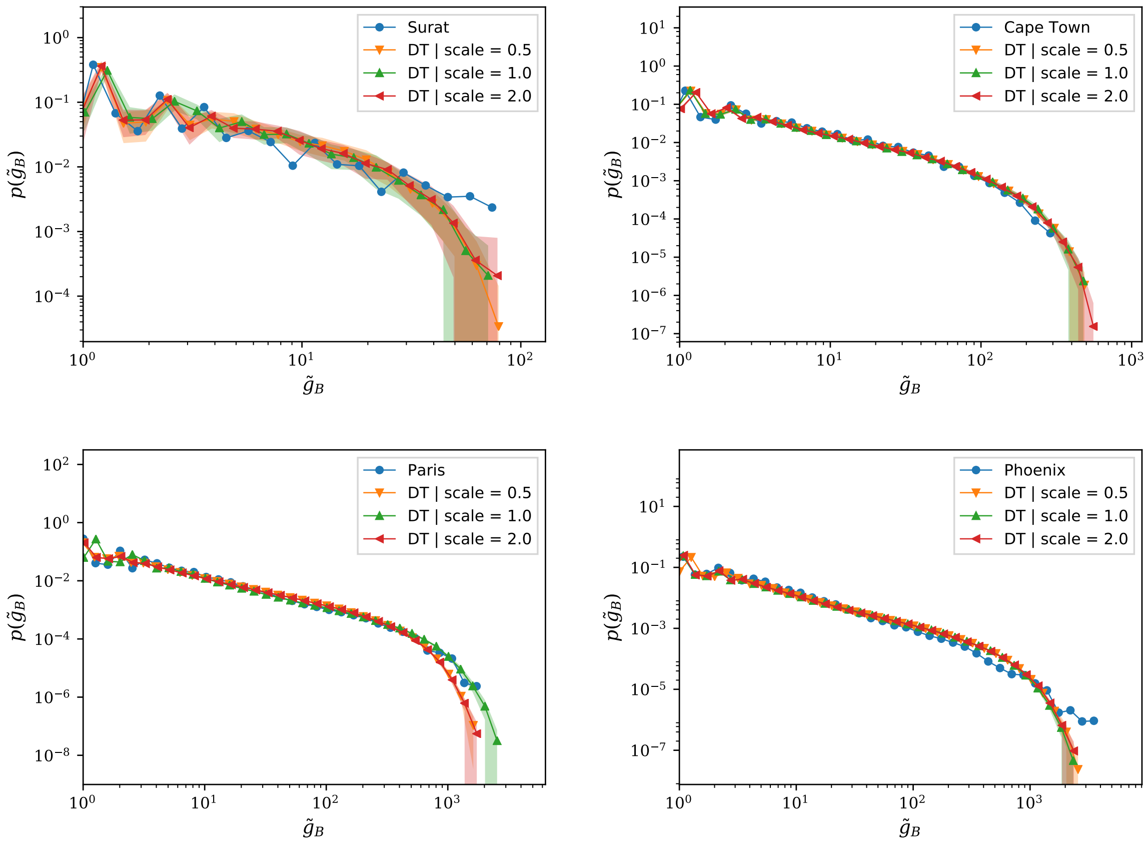


Figure S9: Tails of the BC distributions for selected cities and their corresponding DT for different grid-sizes, having the effect of changing the area and therefore the density of nodes $N/A$. Shown are the results for half and twice the original areas.

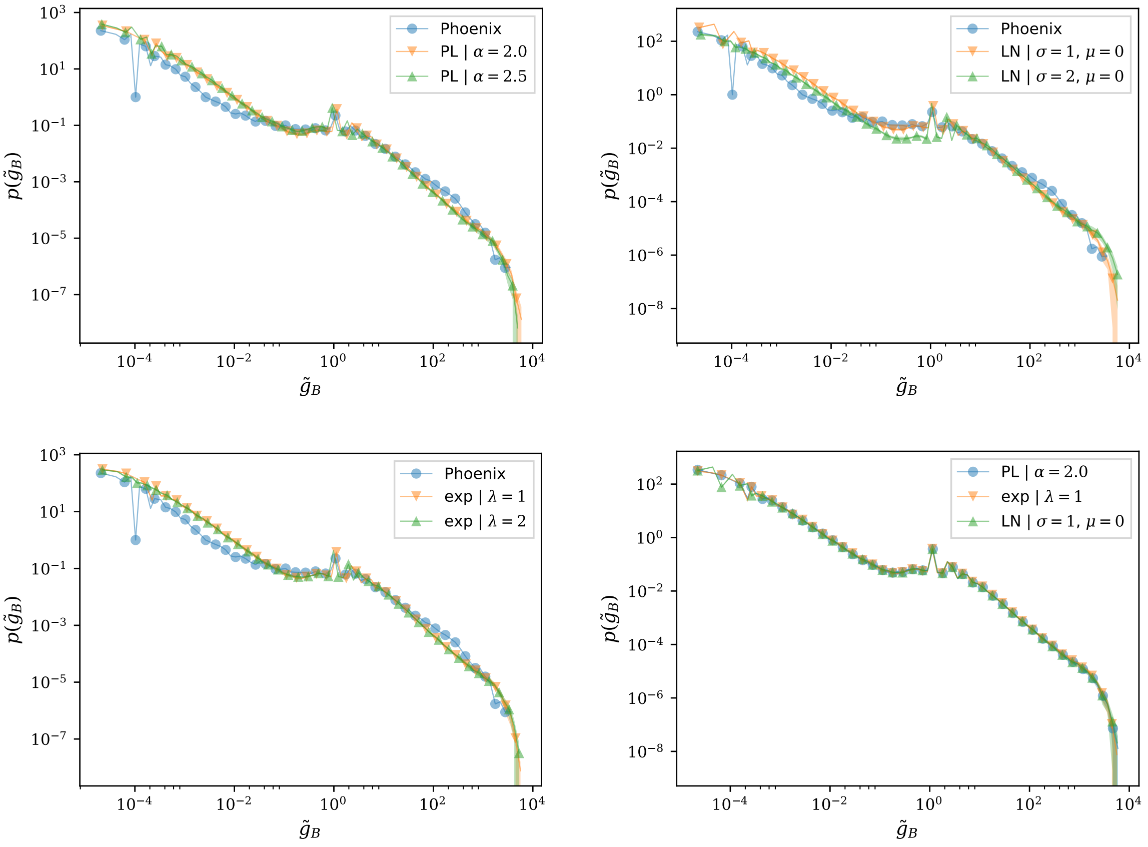


Figure S10: Distribution of $\tilde{g}_B$ for the Phoenix street network, with edge weights generated randomly from multiple families of distributions; power law (PL), exponential (exp) and log normal (LN). The bottom right plot shows three different weight distributions leading to an identical BC profile.

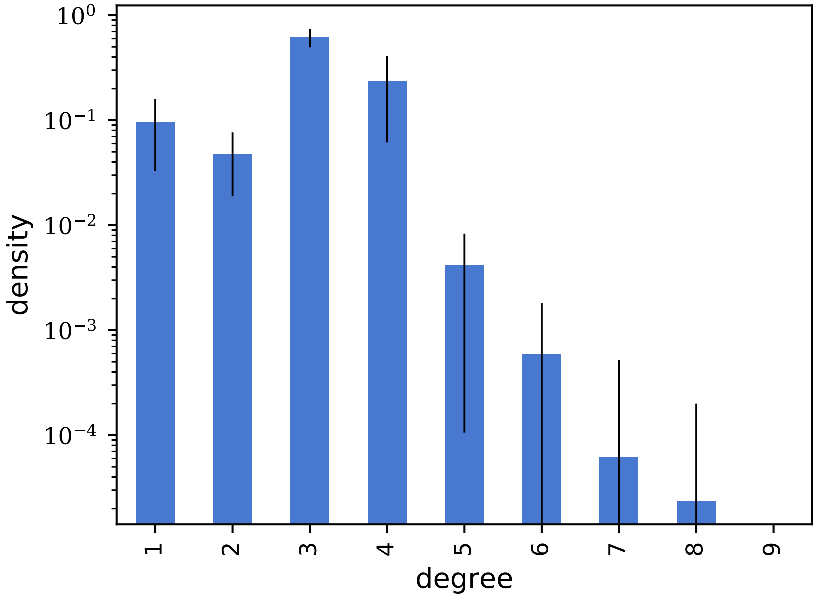


Figure S11: Degree distribution of streets networks averaged over different cities. The length of the black line corresponds to the standard deviation across the cities.

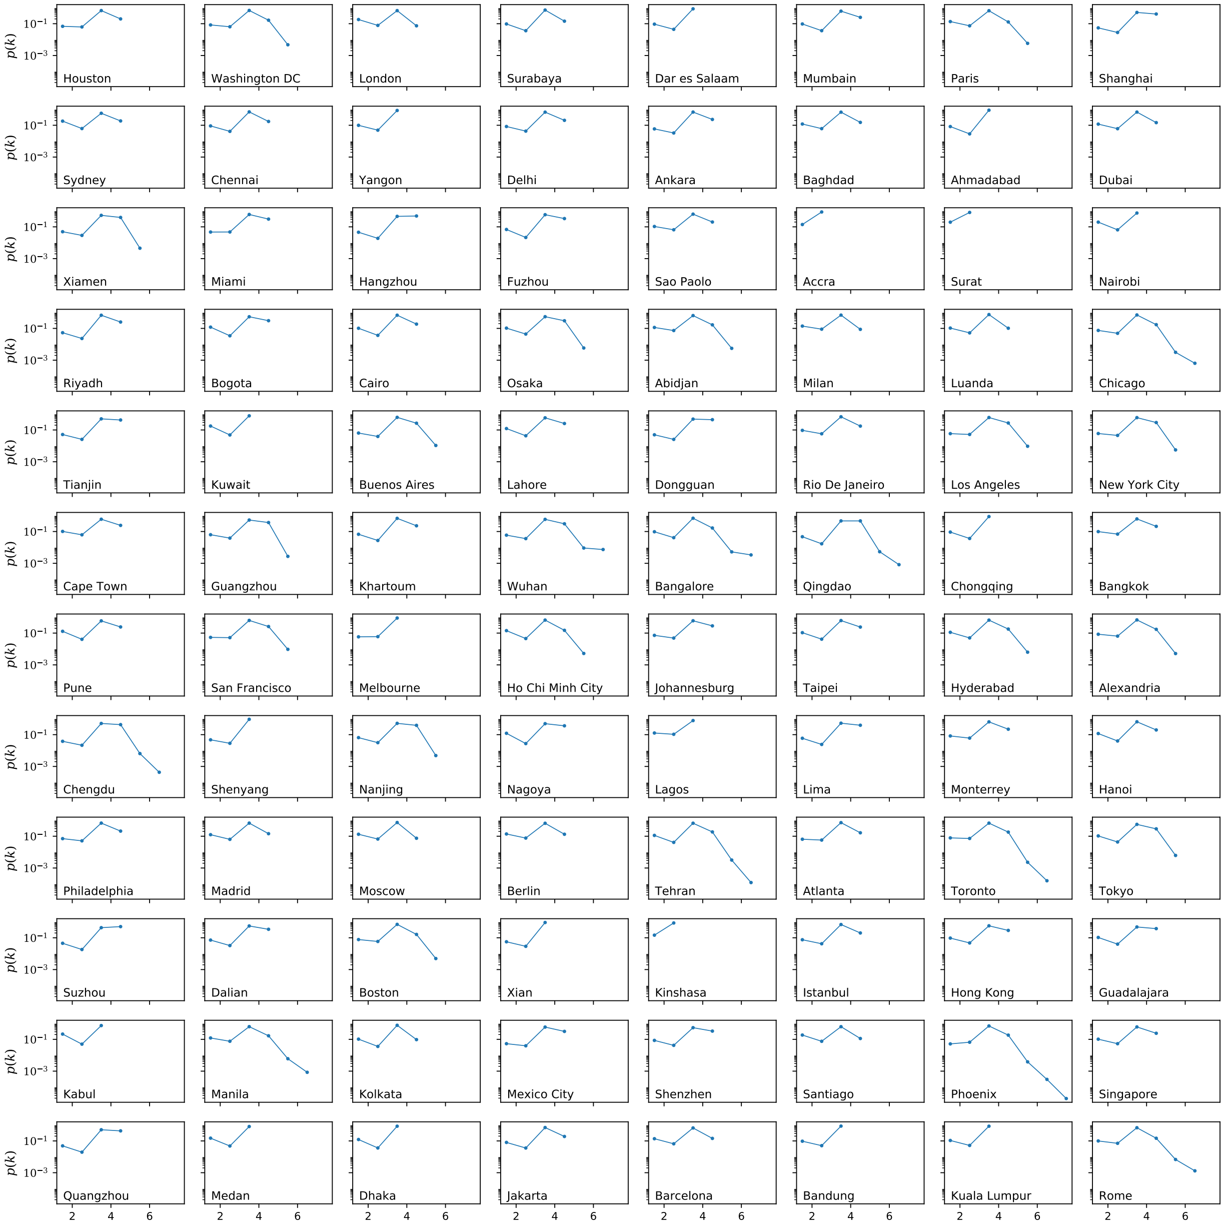


Figure S12: Degree distribution for each individual city, in no particular order.

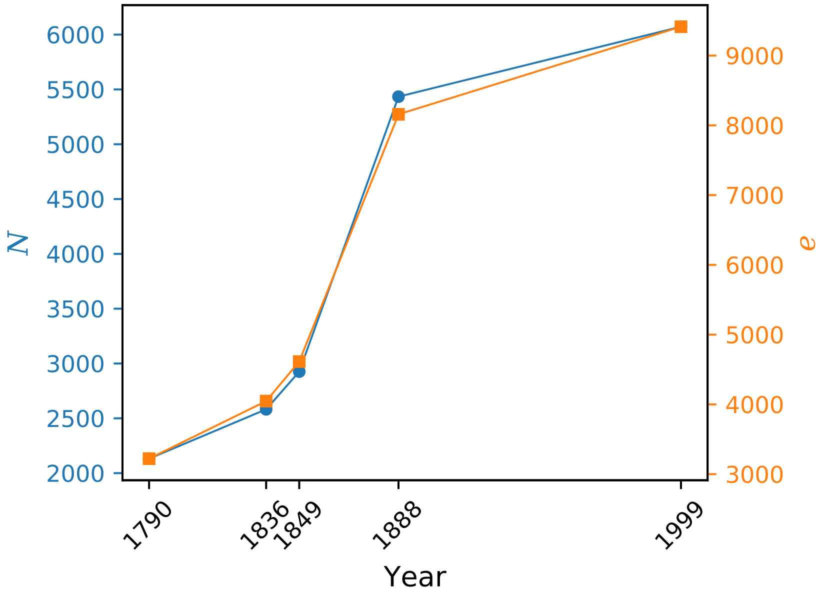


Figure S13: Evolution of the 1789 portion of the Paris street network over a period of approximately 200 years in terms of the number of nodes $N$ and edges $e$. The edge-density is roughly constant, given that nodes and edges grow at the same rate.

## S3 Betweenness centrality of the fastest travel routes

In addition to the full street networks, we also analyzed subsets of the networks corresponding to the fastest travel routes connecting thousands of origin and destination points in the cities. This was motivated by the fact that the fastest routes encapsulate additional dimensions of the underlying road infrastructure such as road capacities and speeds limits. The analysis was conducted on 15 cities sampled from small, mid-sized and large urban areas.

The fastest travel routes were extracted as following: for each city we generated 36 points assigned along the circumferences of circles of 2km, 5km, 10km, 15km, 20km and 30km radii from the city center and spaced at multiples of 10° and enumerated over all OD pairs by connecting the 36 points at a given radius $r$ for a total of $6 \times \binom{36}{2} = 3780$ total OD pairs. We then queried the OpenStreetMap routing API and requested the *fastest* routes connecting each OD pair. The fastest routes are generated by the OSM routing service based on the roads' metadata such as speed limits and road types (e.g., motorway vs. residential), reflecting planning choice and route preferences.

To avoid the influence of unfeasible starting or destination points generated by our method, we discarded from our data the routes whose actual starting or destination points—i.e., the coordinates returned by the OSM API as the starting or ending points of a route—were more than 1km off from the queries point. Moreover, we also excluded those routes whose lengths are longer than $3s + 1km$, where $s$ is the geodesic distance between the origin and destination points. This procedure is the same adopted in [3]. The roads that appeared in at least one of the remaining suggested routes were selected. The networks were then constructed in the same way as we did for the full set of streets.

Table S3 shows the summary statistics for the fastest travel routes in comparison to the complete road data. For the largest cities, the fastest routes correspond to only a small fraction of the overall networks ($\sim$ 10%), while in small urban areas, the fastest routes encompass large fractions of the road infrastructure($\sim$ 40%). Despite this variability, the BC distributions of the fastest route networks exhibit exactly the same scaling properties seen for the full street network as seen in Fig. S14.

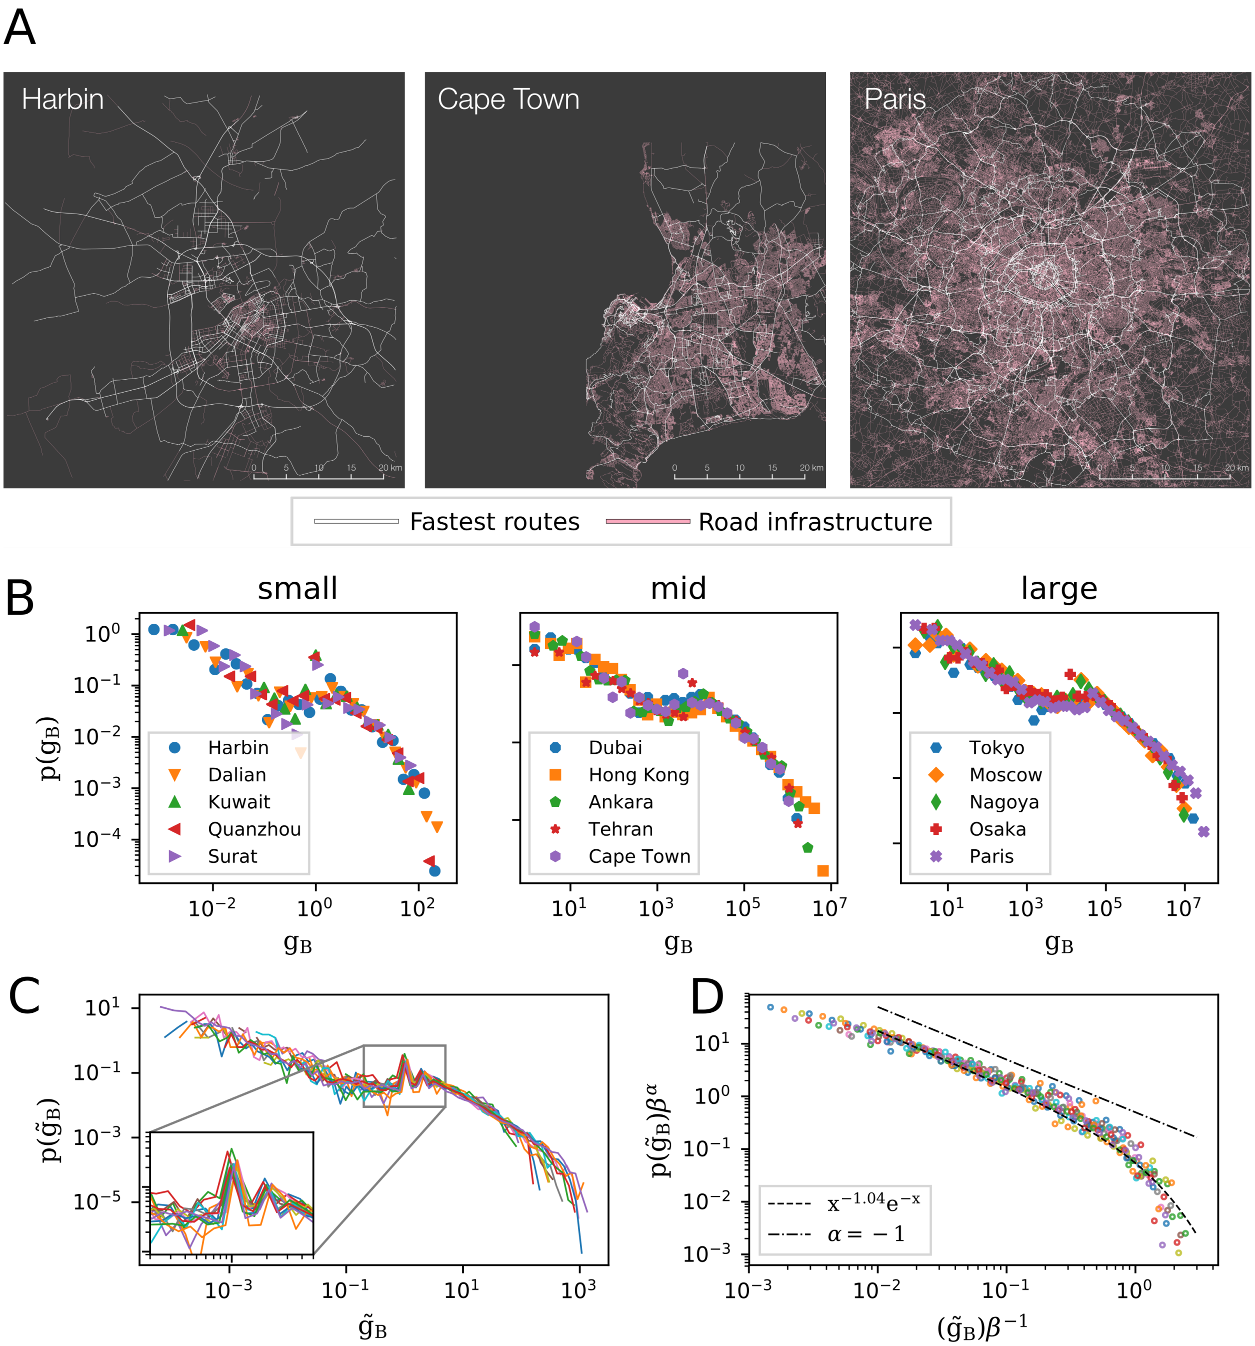


Figure S14: Betweenness centrality of fastest travel routes. (A) The fastest route network (white) overlaid on the full street network (light red) for three different cities chosen from each class (small, mid, large) (B) The BC distribution of the fastest routes exhibit the same properties of the complete streets networks, in spite of their constituting a fraction of the original networks (Table S3). (C) The rescaled BC distribution ($\tilde{g}_b$) collapse on to a single curve with a unique bump at $\tilde{g}_b = 1$ separating the two regimes. (D) Rescaling with respect to $\beta$ results in a collapse of the tails, with an exponent $\alpha \approx 1.04$.

Table S3: Summary statistics for streets networks lying in the fastest travel routes for 15 cities. $N_{routes}$ corresponds to the total number of travel routes obtained for each city that lie on the fastest paths. $\ell$ denotes the total length of the roads systems we analyzed whereas $\ell_{routes}$ denotes the lengths of the roads that were part of the fastest travel routes. The ratio $\ell_{routes}/\ell$ represents the fraction of the total road length corresponding to the fastest routes. $V$ and $V_{routes}$ represent the number of nodes in the original and in the routes networks respectively while $E$ and $E_{routes}$ denote the number of edges in the respective networks.

| City | $N_{routes}$ | $\ell$ (km) | $\ell_{routes}$ (km) | $\ell_{routes}/\ell$ | $V$ | $E$ | $V_{routes}$ | $E_{routes}$ |
|---|---|---|---|---|---|---|---|---|
| Tokyo | 3,540 | 77,087.06 | 5,018.89 | 0.07 | 612,418 | 976,040 | 18,991 | 23,930 |
| Nagoya | 3,725 | 52,523.96 | 4,618.46 | 0.09 | 300,588 | 496,495 | 11,763 | 15,037 |
| Paris | 3,780 | 46,319.14 | 4,551.87 | 0.10 | 279,072 | 425,108 | 22,435 | 27,186 |
| Osaka | 3,305 | 46,049.61 | 4,572.42 | 0.10 | 292,855 | 469,333 | 13,043 | 17,018 |
| Moscow | 3,710 | 43,845.49 | 3,253.94 | 0.07 | 307,472 | 482,217 | 10,587 | 12,314 |
| Hong Kong | 3,004 | 14,437.54 | 2,392.11 | 0.17 | 62,451 | 96,059 | 6,867 | 8,415 |
| Cape Town | 1,683 | 14,301.90 | 1,758.95 | 0.12 | 52,096 | 78,827 | 3,784 | 4,481 |
| Dubai | 2,369 | 14,196.70 | 2,285.92 | 0.16 | 62,559 | 91,822 | 4,747 | 6,394 |
| Tehran | 3,245 | 13,285.97 | 2,994.92 | 0.23 | 57,177 | 88,127 | 5,758 | 7,608 |
| Ankara | 3,326 | 12,632.22 | 2,806.72 | 0.22 | 61,133 | 95,797 | 5,805 | 7,650 |
| Quanzhou | 2,446 | 3,879.01 | 2,034.42 | 0.52 | 3,774 | 6,189 | 1,713 | 2,340 |
| Harbin | 2,582 | 3,806.71 | 1,883.63 | 0.49 | 6,074 | 9,990 | 2,106 | 2,840 |
| Dalian | 1,732 | 2,909.62 | 1,252.77 | 0.43 | 5,654 | 9,122 | 1,960 | 2,604 |
| Surat | 2,672 | 2,161.52 | 1,093.23 | 0.51 | 3,349 | 5,020 | 1,052 | 1,365 |
| Kuwait | 1,237 | 2,084.75 | 891.43 | 0.43 | 4,593 | 6,501 | 585 | 778 |


## Acknowledgements

Map data copyrighted by OpenStreetMap contributors and available from `www.openstreetmap.org`.


## References


[1] OpenStreetMap contributors. Planet dump retrieved from https://planet.osm.org . `https://www.openstreetmap.org` (2017).

[2] Clauset, A., Shalizi, C. R. & Newman, M. E. J. Power-law distributions in empirical data. *SIAM review* **51**, 661–703 (2009).

[3] Lee, M., Barbosa, H., Youn, H., Holme, P. & Ghoshal, G. Morphology of travel routes and the organization of cities. *Nature communications* **8**, 2229 (2017).
